# Supplementary material for: GSN: Generalisable Segmentation in Neural Radiance Field
Source: arXiv:2402.04632 source file (2024-02-07)
Supplement: Supplementary file 1 [file supp_moreclip.tex]

\begin{figure*}[!ht]
    \begin{minipage}{0.24\linewidth}
        \centering
        \begin{tikzpicture}
            \node[anchor=south west,inner sep=0] (image) at (0,0) {\includegraphics[width=\textwidth]{assets/images/supplementary/moreclip/cake000.png}};
        \end{tikzpicture}
    \end{minipage}
    \begin{minipage}{0.24\linewidth}
        \centering
        \begin{tikzpicture}
            \node[anchor=south west,inner sep=0] (image) at (0,0) {\includegraphics[width=\textwidth]{assets/images/supplementary/moreclip/a piece of cake.png}};
        \end{tikzpicture}
    \end{minipage}
    \begin{minipage}{0.24\linewidth}
        \centering
        \begin{tikzpicture}
            \node[anchor=south west,inner sep=0] (image) at (0,0) {\includegraphics[width=\textwidth]{assets/images/supplementary/moreclip/steel_spoon.png}};
        \end{tikzpicture}
    \end{minipage}
    \begin{minipage}{0.24\linewidth}
        \centering
        \begin{tikzpicture}
            \node[anchor=south west,inner sep=0] (image) at (0,0) {\includegraphics[width=\textwidth]{assets/images/supplementary/moreclip/plate.png}};
        \end{tikzpicture}
    \end{minipage}
    
    \caption{\label{fig:supp_moreclip} In this figure, we show more results on a scene containing many objects. The first image shows the ground truth image of the scene. The next three images show the heat-map that we get when we give the text prompts {\em a piece of cake}, {\em a spoon}, and {\em a plate} respectively.}

\end{figure*}
